# Supplementary material for: Validity of Markovian modeling for transient memory-dependent epidemic dynamics
Source: arXiv:2306.16864 source file (2023-07-04)
Supplement: Supplementary file 1 [file SI___Validity_of_Markovian_modeling_for_transient_memory_dependent_epidemic_dynamics.pdf]

Supplementary Information for

# Validity of Markovian modeling for transient memory-dependent epidemic dynamics

Mi Feng, Liang Tian, Ying-Cheng Lai, and Changsong Zhou

Corresponding authors: Liang Tian (liangtian@hkbu.edu.hk) and Changsong Zhou (cszhou@hkbu.edu.hk)

## CONTENTS

Supplementary Note 1. Transformation from non-Markovian to Markovian theory 2

Supplementary Note 2. Derivation of steady-state equivalence 2

Supplementary Note 3. Derivation of transient-state equivalence 4

Supplementary Note 4. The impact of distribution shape on the Markovian average generation(removal) time in transient-state equivalence 4

Supplementary Note 5. Impact of distribution shape on the transmission speed 5

Supplementary Note 6. Analysis of percentile selection 7

References 9

## Supplementary Note 1. TRANSFORMATION FROM NON-MARKOVIAN TO MARKOVIAN THEORY

We set infection and removal time distributions as exponential distributions:

$$\psi_{\rm inf}(\tau) = \gamma e^{-\gamma\tau}, \tag{S1.1}$$

$$\psi_{\rm inf}(\tau) = \mu e^{-\mu\tau}, \tag{S1.2}$$

where their hazard functions satisfy $\omega_{\rm inf}(\tau) = \gamma$ and $\omega_{\rm rem}(\tau) = \mu$, and their survival functions can be expressed as $\Psi_{\rm inf}(\tau) = e^{-\gamma\tau}$, $\Psi_{\rm rem}(\tau) = e^{-\mu\tau}$. Substituting Eqs. (S1.1–S1.2) into Eqs. (1–3) in the main text, we obtain:

$$\frac{ds_l(t)}{dt} = -s_l(t)k\sum_{m=1}^{n} A_{lm}p_m \int_0^t \gamma e^{-\mu(t-t')}dc_m(t'), \tag{S1.3}$$

$$i_l(t) = \int_0^t e^{-\mu(t-t')}dc_l(t'), \tag{S1.4}$$

$$r_l(t) = \int_0^t [1 - e^{-\mu(t-t')}]dc_l(t'). \tag{S1.5}$$

Substituting Eq. (S1.4) into Eq. (S1.3) yields

$$\frac{ds_l(t)}{dt} = -s_l(t)k\gamma\sum_{m=1}^{n} A_{lm}p_m i_m(t). \tag{S1.6}$$

Taking the derivative of Eq. (S1.4) gives

$$\frac{di_l(t)}{dt} = \frac{dc_l(t)}{dt} - \mu\int_0^t e^{-\mu(t-t')}dc_l(t').$$

Since $dc_l(t)/dt = -ds_l(t)/dt$, we obtain

$$\frac{di_l(t)}{dt} = s_l(t)k\gamma\sum_{m=1}^{n} A_{lm}p_m i_m(t) - \mu i_l(t), \tag{S1.7}$$

Taking the derivative of Eq. (S1.5) gives

$$\frac{dr_l(t)}{dt} = \mu\int_0^t e^{-\mu(t-t')}dc_l(t').$$

We have

$$\frac{dr_l(t)}{dt} = \mu i_l(t), \tag{S1.8}$$

## Supplementary Note 2. DERIVATION OF STEADY-STATE EQUIVALENCE

Equation (1) in the main text can be rewritten as

$$\frac{d\ln s_l(t)}{dt} = -k\sum_{m=1}^{n} A_{lm}p_m \int_0^t \omega_{\rm inf}(t-t')\Psi_{\rm rem}(t-t')dc_m(t'). \tag{S2.9}$$

Integrating both sides of the equation from 0 to infinity yields the following relationship:

$$\ln \tilde{s}_l - \ln \acute{s}_l = -k \sum_{m=1}^{n} A_{lm} p_m \int_0^{+\infty} \int_0^{t} \omega_{\text{inf}}(t-t')\Psi_{\text{rem}}(t-t')dc_m(t')dt. \tag{S2.10}$$

Exchanging the order of integration with respect to $t$ and $t'$, we obtain

$$\ln \tilde{s}_l - \ln \acute{s}_l = -k \sum_{m=1}^{n} A_{lm} p_m \int_0^{+\infty} \int_{t'}^{+\infty} \omega_{\text{inf}}(t-t')\Psi_{\text{rem}}(t-t')dtdc_m(t'), \tag{S2.11}$$

or

$$\ln \tilde{s}_l - \ln \acute{s}_l = -k \sum_{m=1}^{n} A_{lm} p_m \lambda_{\text{eff}} \int_0^{+\infty} dc_m(t), \tag{S2.12}$$

where the $\lambda_{\text{eff}}$ is the effective infection rate given by

$$\lambda_{\text{eff}} = \int_0^{+\infty} \omega_{\text{inf}}(\tau)\Psi_{\text{rem}}(\tau)d\tau. \tag{S2.13}$$

The physical meaning of $dc_m(t)$ is the new infected fraction in age group $m$ at time $t$, which can further spread the infection to others. So the value of $dc_m(0)$ should be considered as the fraction of infection seeds, where the initial removed fraction are not taken into account. We thus have $\int_0^{+\infty} dc_m(t) = \tilde{c}_m - \acute{r}_m$ and

$$\ln \tilde{s}_l - \ln \acute{s}_l = -k \sum_{m=1}^{n} A_{lm} p_m \lambda_{\text{eff}} (\tilde{c}_m - \acute{r}_m). \tag{S2.14}$$

Because all the infected individuals will eventually be removed, we have $\tilde{c}_l = \tilde{r}_l$. We obtain the following relationship:

$$\tilde{s}_l = \acute{s}_l e^{-\lambda_{\text{eff}} \sum_{m=0}^{n} k A_{lm} p_m (\tilde{r}_m - \acute{r}_l)}. \tag{S2.15}$$

For the steady state in a Markovian framework, we have $\psi_{\text{inf}}(\tau) = \gamma e^{-\gamma\tau}$ and $\psi_{\text{rem}}(\tau) = \mu e^{-\mu\tau}$, which lead to $\omega_{\text{inf}}(\tau) = \gamma$ and $\Psi_{\text{rem}}(\tau) = e^{-\mu\tau}$, respectively. Substituting these into Eq. (S2.13) gives

$$\lambda_{\text{eff}} = \frac{\gamma}{\mu}. \tag{S2.16}$$

As for steady state, in the thermodynamic limit where the total population size tends to infinity, the calculation of $\lambda_{\text{eff}}$ reveal the existence of a critical point $\lambda_{\text{eff}}^{\text{c}}$ [1, 2]. Below this critical point, the system approaches a typical non-equilibrium absorbing phase, and the final cumulative infection (or removal) approaches zero. Above the critical point, the system reaches an active phase and the final cumulative infection (or removal) has a nonzero average value. The critical point is related to the contact pattern of the dynamics and can be calculated using the relation $\lambda_{\text{eff}}^{\text{c}} = 1/\Lambda_{\max}$, where $\Lambda_{\max}$ is the maximum eigenvalue of the matrix $k\boldsymbol{A} \circ \boldsymbol{p}$, where $\circ$ denotes a row-wise Hadamard product between a matrix and a vector. This relationship enables us to calculate the basic reproduction number $R_0$ as:

$$R_0 = \lambda_{\text{eff}} \Lambda_{\max}, \tag{S2.17}$$

which divides the absorbing and active phases at $R_0 = 1$. Note that $\Lambda_{\max}$ is calculated under the condition that all individuals are susceptible, so $R_0$ is a measure of the average number of secondary infections resulting from a single infected individual during the course of their infectious

period in a fully susceptible population. Since $R_0$ is calculated as the product of a coefficient and the effective infection rate $\lambda_{\text{eff}}$, it is interchangeable with $\lambda_{\text{eff}}$ when describing the dynamics of a system and calculating the steady state, indicating that identical values of $R_0$ will result in the same steady state in certain systems.

## Supplementary Note 3. DERIVATION OF TRANSIENT-STATE EQUIVALENCE

Integrating both sides of Eq. (S2.9) from 0 to $t$ yields the following relationship:

$$\ln s_l(t) - \ln \acute{s}_l = -k \sum_{m=1}^{n} A_{lm} p_m \int_0^t \int_0^{t'} \omega_{\text{inf}}(t'-t'')\Psi_{\text{rem}}(t'-t'')dc_m(t'')dt'. \tag{S3.18}$$

Exchanging the order of integration with respect to $t'$ and $t''$, we obtain

$$\ln s_l(t) - \ln \acute{s}_l = -k \sum_{m=1}^{n} A_{lm} p_m \int_0^t \int_{t''}^{t} \omega_{\text{inf}}(t'-t'')\Psi_{\text{rem}}(t'-t'')dt'dc_m(t''). \tag{S3.19}$$

For $\omega_{\text{inf}}(\tau) \propto \omega_{\text{rem}}(\tau)$, which gives that $\omega_{\text{inf}}(\tau) = \lambda_{\text{eff}}\omega_{\text{rem}}(\tau)$, we get

$$\begin{aligned} \ln s_l(t) - \ln \acute{s}_l &= -k \sum_{m=1}^{n} A_{lm} p_m \lambda_{\text{eff}} \int_0^t [1 - \Psi_{\text{rem}}(t-t'')]dc_m(t'') \\ &= -k \sum_{m=1}^{n} A_{lm} p_m \lambda_{\text{eff}} (r_m(t) - \acute{r}_m), \end{aligned} \tag{S3.20}$$

leading to

$$s_l(t) = \acute{s}_l e^{-\lambda_{\text{eff}} \sum_{m=0}^{n} k A_{lm} p_m [r_m(t) - \acute{r}_m]}. \tag{S3.21}$$

According to the definitions of average generation and removal times, $\omega_{\text{inf}}(\tau) \propto \omega_{\text{rem}}(\tau)$ will further result in $T_{\text{gen}} = T_{\text{rem}}$. For some distributions, e.g., Weibull distribution, we obtain the relationship $\omega_{\text{inf}}(\tau) \propto \omega_{\text{rem}}(\tau) \Leftrightarrow T_{\text{gen}} = T_{\text{rem}}$.

Because the Weibull distribution is a highly adaptable distribution capable of approximating various other distributions, such as the exponential, Rayleigh, and log-normal distributions, the flexibility makes it a valuable tool for modeling a diverse range of phenomena and a practical choice for many real-world applications. Making the mathematical assumption of Weibull distributions does not result in significant differences compared to a general scenario, and by substituting ”=” in Eq. (S3.21) with ”$\simeq$”, Eq. (11) in the main text can be applied to situations beyond those that assume Weibull distributions.

## Supplementary Note 4. THE IMPACT OF DISTRIBUTION SHAPE ON THE MARKOVIAN AVERAGE GENERATION(REMOVAL) TIME IN TRANSIENT-STATE EQUIVALENCE

To study how the distribution shape in the non-Markovian dynamic affects the average generation (removal) time in the transient-equivalent Markovian one, we keep the values of $T_{\text{gen}}$ and $T_{\text{rem}}$ constant and ensure that they are both equal to 7 in a non-Markovian transmission. We use

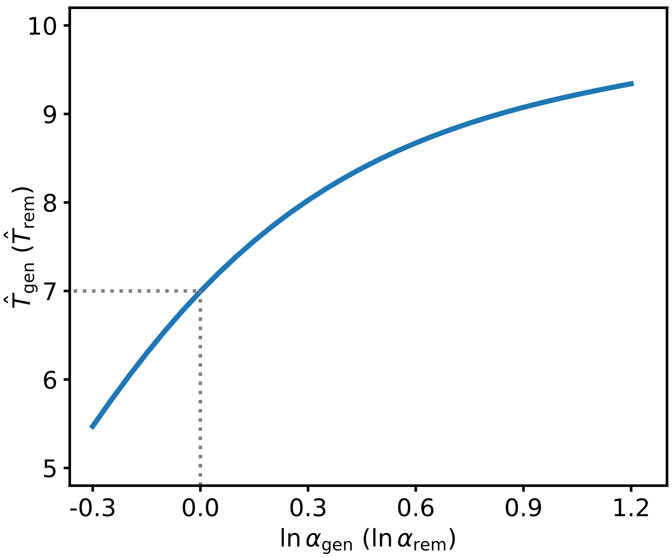


FIG. S1. Average generation time $\hat{T}_{\mathrm{gen}}$ and average removal time $\hat{T}_{\mathrm{rem}}$ increase as the shape parameter $\ln \alpha_{\mathrm{gen}}$ and $\ln \alpha_{\mathrm{rem}}$ increase. The dotted lines in the graph indicate that only when $\alpha_{\mathrm{gen}} = \alpha_{\mathrm{rem}} = 1$ can an equality in the average generation (removal) times be achieved.

the Weibull distributions for both $\psi_{\mathrm{gen}}(\tau)$ and $\psi_{\mathrm{rem}}(\tau)$, so $\psi_{\mathrm{inf}}(\tau)$ must follow a Weibull distribution to achieve that. Meanwhile, their shape parameters, $\alpha_{\mathrm{inf}}$, $\alpha_{\mathrm{rem}}$, and $\alpha_{\mathrm{gen}}$, are also needed to be equal. We vary the shape parameters from less than one to greater than one and calculate the corresponding average generation and removal times, denoted as $\hat{T}_{\mathrm{gen}}$ and $\hat{T}_{\mathrm{rem}}$, respectively, for the equivalent Markovian theory. Supplementary Fig. S1 shows that, when the shape parameter is less than one, $\hat{T}_{\mathrm{gen}}$ and $\hat{T}_{\mathrm{rem}}$ in the equivalent Markovian theory are smaller than those in the non-Markovian transmission. When the shape parameter is greater than one, $\hat{T}_{\mathrm{gen}}$ and $\hat{T}_{\mathrm{rem}}$ in the equivalent Markovian theory are greater than those in the non-Markovian transmission. Only when the non-Markovian transmission is reduced to a Markovian one, i.e., $\alpha_{\mathrm{gen}} = \alpha_{\mathrm{rem}} = 1$ , can we achieve equality of the average generation (removal) times. In the next, we analyze this phenomenon mathematically.

## Supplementary Note 5. IMPACT OF DISTRIBUTION SHAPE ON THE TRANSMISSION SPEED

To mathematically illustrate how the shape of the generation time distribution affects the transmission speed, we assume $\psi_{\mathrm{gen}}(\tau)$ as a gamma distribution:

$$\psi_{\mathrm{gen}}(\tau) = \frac{1}{\Gamma(\alpha_{\mathrm{gen}})\beta_{\mathrm{gen}}^{\alpha_{\mathrm{gen}}}} \tau^{\alpha_{\mathrm{gen}}-1} e^{-\frac{\tau}{\beta_{\mathrm{gen}}}} \tag{S5.22}$$

where $\alpha_{\mathrm{gen}}$ and $\beta_{\mathrm{gen}}$ are, respectively, the shape and scale parameters, and the average generation time satisfies $T_{\mathrm{gen}} = \alpha_{\mathrm{gen}}\beta_{\mathrm{gen}}$. The primary reason for choosing the gamma distribution for the generation time is the analytical tractability of the Euler-Lotka equation in this case. Furthermore, the gamma and Weibull distributions share similar characteristics, making it reasonable to apply

the results obtained with the gamma distribution to the Weibull distribution. The calculation is also applicable to other distributions.

Substituting the gamma distribution into Euler-Lotka Equation, i.e.,

$$1 = R_0 \int_0^{+\infty} e^{-g\tau}\psi_{\text{gen}}(\tau)d\tau. \tag{S5.23}$$

we obtain

$$\frac{1}{R_0} = \left(\frac{1}{1+\beta_{\text{gen}}g}\right)^{\alpha_{\text{gen}}} \tag{S5.24}$$

We identify an transient equivalent memoryless transmission with infection rate $\gamma$ and removal rate $\mu$. The growth rate can be obtained as $g = \mu(R_0 - 1)$. Substituting it into Eq. (S5.24) we get

$$\frac{1}{\mu} = \frac{R_0 - 1}{\alpha_{\text{gen}}(R_0^{1/\alpha_{\text{gen}}} - 1)} \cdot \alpha_{\text{gen}}\beta_{\text{gen}},$$

which gives

$$T^*_{\text{gen}} = \frac{R_0 - 1}{\alpha_{\text{gen}}(R_0^{1/\alpha_{\text{gen}}} - 1)} \cdot T_{\text{gen}}. \tag{S5.25}$$

Where $T^*_{\text{gen}}$ and $T_{\text{gen}}$ are, respectively, the average generation times of the memoryless and memory-dependent transmission dynamics. In this case, the average generation time of the equivalent memoryless transmission is affected by both the reproductive number and the shape of the generation distribution.

More specifically, we consider a fixed $R_0 > 1$ and $T_{\text{gen}}$ and aim to show that the value of $T^*_{\text{gen}}$ will increase as $\alpha_{\text{gen}}$ increases. To this end, we set $x = 1/\alpha_{\text{gen}}$ and define a function

$$h(x) = \frac{R_0^x - 1}{x}$$

that encodes the denominator of the right-hand side of Eq. (S5.25). To prove that $h(x)$ is a monotonically increasing function, we calculate the derivative of $h(x)$:

$$h'(x) = \frac{(x\ln R_0 - 1)R_0^x + 1}{x^2}. \tag{S5.26}$$

To prove that $h'(x)$ is positive for $x > 0$, we define another function $q(x) = (x\ln R_0 - 1)R_0^x + 1$, where $q(0) = 0$. The derivative of $q(x)$ is:

$$q'(x) = (\ln R_0)^2 x R_0^x. \tag{S5.27}$$

Since $(\ln R_0)^2 > 0$ and $R_0^x > 0$ for $x > 0$, $q(x)$ is a monotonically increasing function for $x > 0$. Consequently, $q(x) > 0$ for $x > 0$. We conclude that $q'(x) > 0$ for $x > 0$ and thus $h'(x) > 0$ for $x > 0$. As a result, $h(x)$ is a monotonically increasing function for $x > 0$. This means that the quantity

$$\frac{R_0 - 1}{\alpha_{\text{gen}}(R_0^{1/\alpha_{\text{gen}}} - 1)}$$

monotonically increases as $\alpha_{\text{gen}}$ gets larger, which implies that $T^*_{\text{gen}}$ increases with an increasing $\alpha_{\text{gen}}$.

## Supplementary Note 6. ANALYSIS OF PERCENTILE SELECTION

The metric $\varepsilon$ serves to quantify the relative deviation of the Markovian curves from their corresponding, more accurate non-Markovian counterparts. The value of $\varepsilon$ can vary depending on the selection of percentiles $\theta$. If the transient-state equivalence holds, and the percentile value $\theta$ increases from 1 to 100, the value of $\varepsilon$ will initially decrease and then increase. Consequently, if the percentile $\theta$ is too small or too large, $\varepsilon$ will become significantly large. To ensure accurate calculations, caution needs to be exercised when selecting an appropriate value of $\theta$.

To better illustrate this phenomenon, we consider a non-Markovian transmission with $T_{\text{gen}} = T_{\text{rem}}$. We identify the corresponding equivalent Markovian transmission, wherein the infection and removal rates in Eqs. (S1.1) and (S1.2) are computed using the Euler-Lotka equation, i.e., Eq. (S5.23). The Euler-Lotka equation presupposes that the number of cumulative infections increases exponentially during the initial phase of an outbreak, and any changes in the fraction of the susceptible population can be ignored during this early stage of transmission. When the percentile $\theta$ is small, the susceptible fraction approximately remains constant in the initial phase of the outbreak. However, only the Markovian theory, given its constant infection and removal rates, can accurately predict the exponential increase. In contrast, the non-Markovian transmission, with its variable infection and removal rates, is not consistent with the exponential increase during the short-term transmission. As the percentile $\theta$ increases, the variability of the infection and removal rate in the infectious period is averaged and the curves will begin to approach the exponential curves. Consequently, at this percentile, the non-Markovian curves closely resembles the Markovian curves. However, as the percentile $\theta$ continues to increase, the two assumptions no longer hold, and the "distance" between the non-Markovian and Markovian transmission will start to increase. Despite this, both types of transmission will reach the same steady state with small deviations, so the approximate equivalence still holds.

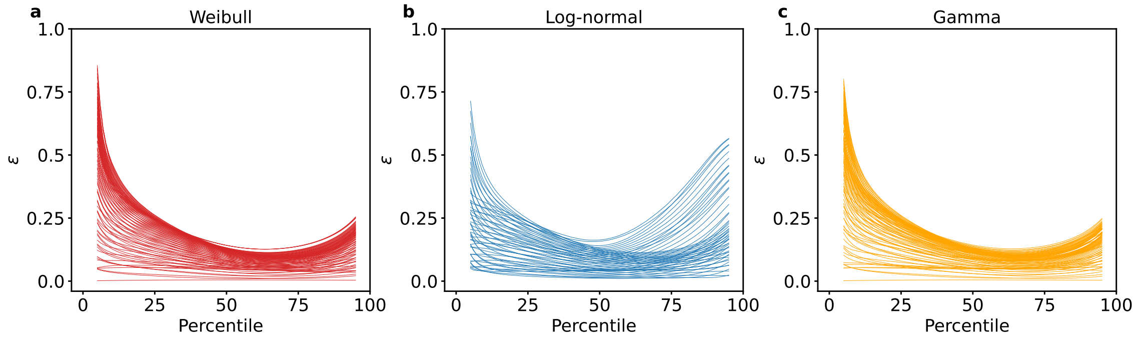


FIG. S2. **a–c**. Relationship between $\varepsilon$ and $\theta$ for a set of non-Markovian transmission models that satisfy $T_{\text{gen}} \simeq T_{\text{rem}}$, with Weibull, log-normal, and gamma time distributions.

As demonstrated in Supplementary Fig. S2, we conducted tests on a set of non-Markovian transmission models that satisfy $T_{\text{gen}} \simeq T_{\text{rem}}$ using Weibull, log-normal, and gamma time distributions. For the majority of the curves, as we change the value of $\theta$, the corresponding value of $\varepsilon$ first decreases and then increases, consistent with our earlier analysis.

In the main text, we select the percentile $\theta$ to be 50. Computations indicate that the minimal value of $\varepsilon$ is achieved when $T_{\text{gen}}$ is equal to $T_{\text{rem}}$. These results demonstrate a good agreement across various time distribution forms and parameter values. Supplementary Fig. S3 illustrates that

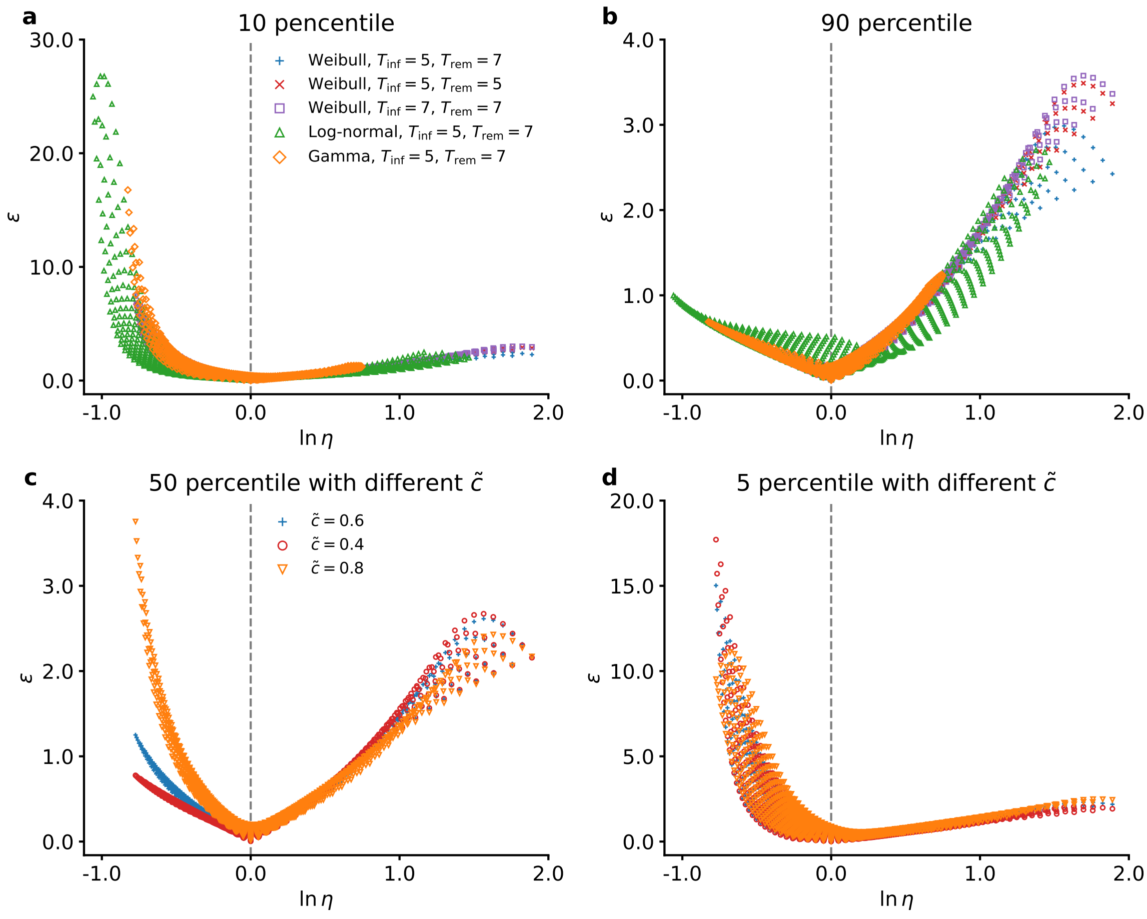


FIG. S3. **a** Results of $\varepsilon$ with respect to $\ln \eta$ for $\theta = 10$. **b** Results of $\varepsilon$ with respect to $\ln \eta$ for $\theta = 90$. **c** Results of $\varepsilon$ with respect to $\ln \eta$ with different values of $\tilde{c}$ for $\theta = 50$. **d** Results of $\varepsilon$ with respect to $\ln \eta$ with different values of $\tilde{c}$ for $\theta = 5$.

the same trend is observed when we modify the percentile from 50 to both 10 and 90. However, note that for $\theta = 10$, although $\varepsilon$ can attain a significantly low value when $T_{\mathrm{gen}} = T_{\mathrm{rem}}$, maintaining the condition $T_{\mathrm{gen}} > T_{\mathrm{rem}}$ also preserves the value of $\varepsilon$ at a relatively low level. In this case, the results with log-normal time distributions become more dispersed for $T_{\mathrm{gen}} < T_{\mathrm{rem}}$ (Supplementary Fig. S3a). Similarly, for $\theta = 90$, the outcomes with log-normal time distribution exhibit increased scattering, even when $T_{\mathrm{gen}}$ is equal to $T_{\mathrm{rem}}$ (Supplementary Fig. S3b).

In the main text, we maintain a constant cumulative infected proportion $\tilde{c}$ of $0.6$ by adjusting the value of $k$ in Eq. (7). We then proceed to investigate the effect of varying $\tilde{c}$ from 0.6 to 0.4 and 0.8, while keeping $\theta$ fixed at 50. Our computations indicate that the curves for $T_{\mathrm{gen}} < T_{\mathrm{rem}}$ do not align with one another (Supplementary Fig. S3c). This discrepancy can be attributed to higher values of $\tilde{c}$ being further from the initial outbreak, resulting in a deviation from the Euler-Lotka equation, even though the $\theta$ values remain the same. When we set the value of $\theta$ to 5 to ensure that all calculations of $\varepsilon$ utilize data from the initial outbreak, the results demonstrate improved agreement across different values of $\tilde{c}$ (Supplementary Fig. S3d).

[1] Wang, Y., Chakrabarti, D., Wang, C. & Faloutsos, C. Epidemic spreading in real networks: An eigenvalue viewpoint. In *22nd International Symposium on Reliable Distributed Systems, 2003. Proceedings.*, 25–34 (IEEE, 2003).

[2] Chakrabarti, D., Wang, Y., Wang, C., Leskovec, J. & Faloutsos, C. Epidemic thresholds in real networks. *ACM Trans. Inf. Syst. Secur.* **10**, 1–26 (2008).
